# Supplementary material for: BooW-VTON: Boosting In-the-Wild Virtual Try-On via Mask-Free Pseudo Data Training
Source: arXiv:2408.06047 source file (2024-11-22)
Supplement: Supplementary file 1 [file Results.tex]

% \clearpage
\section{More Visual Results}
\label{more_results}

% This section presents additional visualization results, including those from four datasets and selected zero-shot examples.

% \subsection{VITON-HD}

\begin{figure*}[h]
    \centering
    % \hspace*{-0.1\textwidth}  
    \includegraphics[width=1\textwidth]{Appendix/images/more_results_hd.jpg}
    \caption{Visualization of comparison results on the VITON-HD test set.
    \label{fig:comparsion_hd}}
\end{figure*}

\begin{figure*}[h]
    \centering
    \includegraphics[width=1.0\textwidth]{Appendix/images/VITONHD_Cross_1.jpg}
    \caption{Additional try-on results on the VITON-HD test set.
    \label{fig:cross_hd}}
\end{figure*}

% \clearpage
% \subsection{DressCode}

\begin{figure*}[h]
    \centering
    % \hspace*{-0.15\textwidth}  
    \includegraphics[width=1\textwidth]{Appendix/images/more_results_dc_upper.jpg}
    \caption{Visualization of comparison results on the DressCode Upper test set.
    \label{fig:com_dc_upper}}
\end{figure*}

\begin{figure*}[h]
    \centering
    % \hspace*{-0.15\textwidth}  
    \includegraphics[width=1\textwidth]{Appendix/images/more_results_dc_lower.jpg}
    \caption{Visualization of comparison results on the DressCode Lower test set.
    \label{fig:com_dc_lower}}
\end{figure*}

\begin{figure*}[h]
    \centering
    % \hspace*{-0.15\textwidth}  
    \includegraphics[width=1\textwidth]{Appendix/images/more_results_dc_dresses.jpg}
    \caption{Visualization of comparison results on the DressCode Dresses test set.
    \label{fig:com_dc_dress}}
\end{figure*}

\begin{figure*}[h]
    \centering
    \includegraphics[width=1.0\textwidth]{Appendix/images/more_results_dc_cross_1.jpg}
    \caption{Cross-Garment type try-on results on the DressCode test set (Part 1).
    \label{fig:dc_cross_1}}
\end{figure*}

\begin{figure*}[h]
    \centering
    \includegraphics[width=1.0\textwidth]{Appendix/images/more_results_dc_cross_2.jpg}
    \caption{Cross-Garment type try-on results on the DressCode test set (Part 2).
    \label{fig:dc_cross_2}}
\end{figure*}

\begin{figure*}[h]
    \centering
    % \hspace*{-0.1\textwidth}  
    \includegraphics[width=1\textwidth]{Appendix/images/more_results_st.jpg}
    \caption{Visualization of comparison results on the StreetVTON test set.
    \label{fig:com_st}}
\end{figure*}

% \clearpage
% \subsection{WildVTON}
% \vspace{-30mm}
\begin{figure*}[h]
    \centering
    % \hspace*{-0.1\textwidth}  
    \includegraphics[width=1\textwidth]{Appendix/images/more_results_wd.jpg}
    \caption{Visualization of comparison results on the WildVTON test set.
    \label{fig:com_wd}}
\end{figure*}

\begin{figure*}[h]
    \centering
    % \hspace*{-0.05\textwidth}  
    \includegraphics[width=1\textwidth]{Appendix/images/Wild_Cross_3.jpg}
    \caption{Cross-Garment type try-on results on the WildVTON test set.
    \label{fig:cross_wd}}
\end{figure*}

BooW-VTON achieves highly realistic and natural in-the-wild try-on results. This realism stems from the preservation of lighting conditions and spatial structures. As shown clearly in Figure \ref{fig:hq_tryon}: In the first row, our try-on results not only retain the details of the subject's skin but also faithfully reproduce the shading on the arm. In the second row, while preserving details across various types of garment, BooW-VTON maintains the influence of the top light source on the entire image. In the third row, BooW-VTON accounts for the model's orientation and leg movement, deforming the clothing accordingly to produce realistic and natural try-on results.
\begin{figure*}[h]
    \centering
    % \hspace*{-0.05\textwidth}  
    \includegraphics[width=1\textwidth]{Appendix/images/more_results_internet.jpg}
    \caption{High-quality in-the-wild try-on results with lighting features and spatial structures.
    \label{fig:hq_tryon}}
\end{figure*}
